# Supplementary material for: A Pilot Design for Observational Studies: Using Abundant Data Thoughtfully
Source: arXiv:1908.09077 ancillary file (2020-08-21)
Supplement: Supplementary file 1 [file Supplementary_Figures.pdf]

# Supplementary Figures

A Pilot Design for Observational Studies: Using Abundant Data Thoughtfully

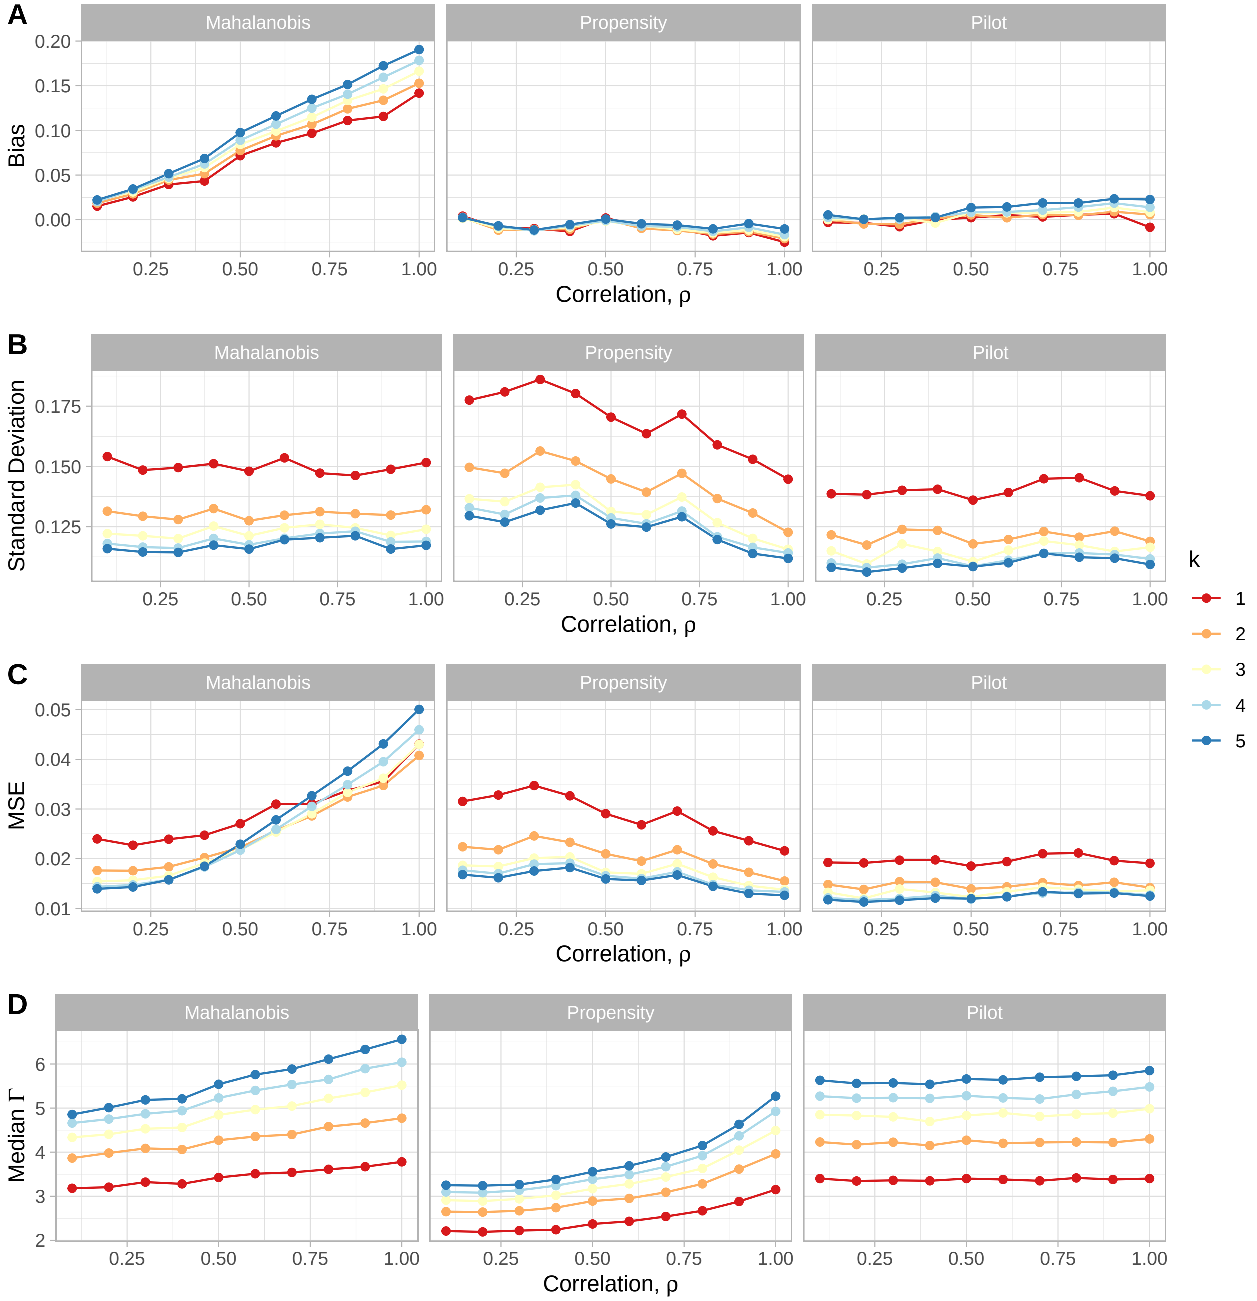


**Supplementary Figure 1:** Bias, standard deviation, MSE and median gamma when the score models were fit with a lasso. All simulation parameters are the same as described in Section 4.2, except that $\phi(X_i) = X_{i1}/2 - 3$, giving more structure to the propensity score so that it could reasonably be fit with a sparsifying model. The regularization penalty for each score model was determined using 10-fold cross validation. In rare cases, the propensity score model with minimum cross-validation error amounted to estimating all non-intercept model coefficients as zero. When this occurred, a very mild ($\lambda = 0.005$) regularization was used as a default, rather than the cross-validation optimum.

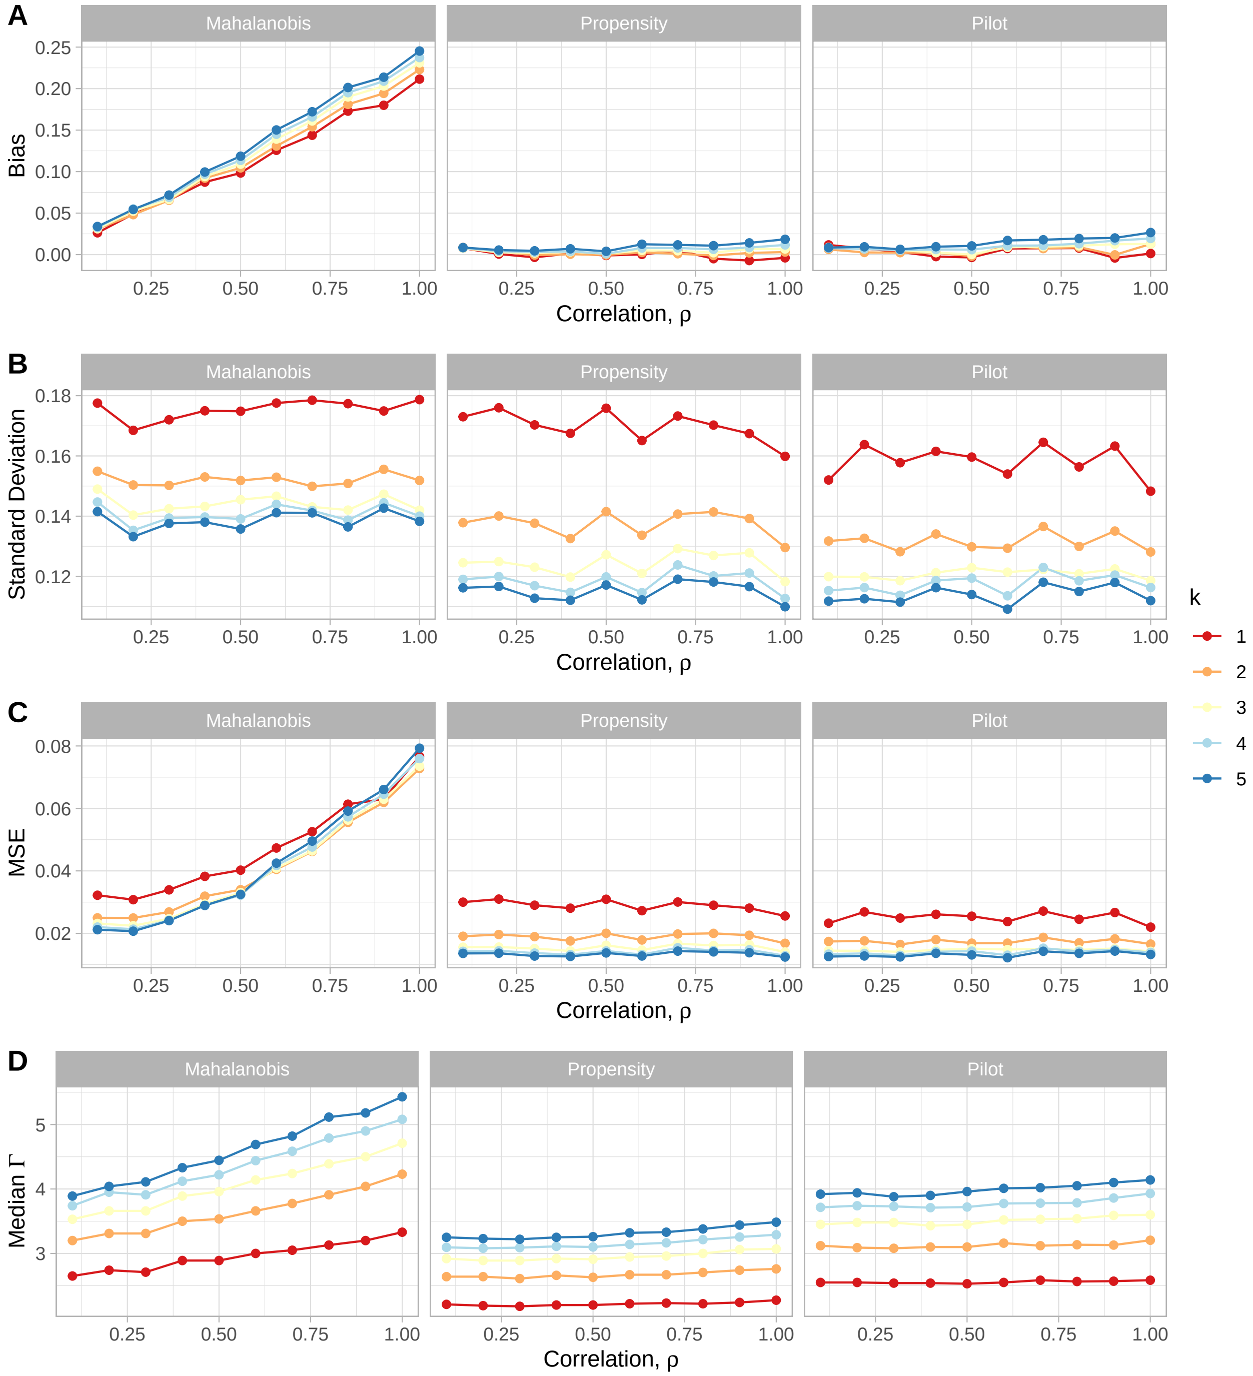


**Supplementary Figure 2:** Bias, standard deviation, MSE, and median Γ of matching estimators when the number of uninformative covariates is increased. All simulation parameters are the same as described in Section 4.2, except that the number of covariates, $p$, is increased to 50.

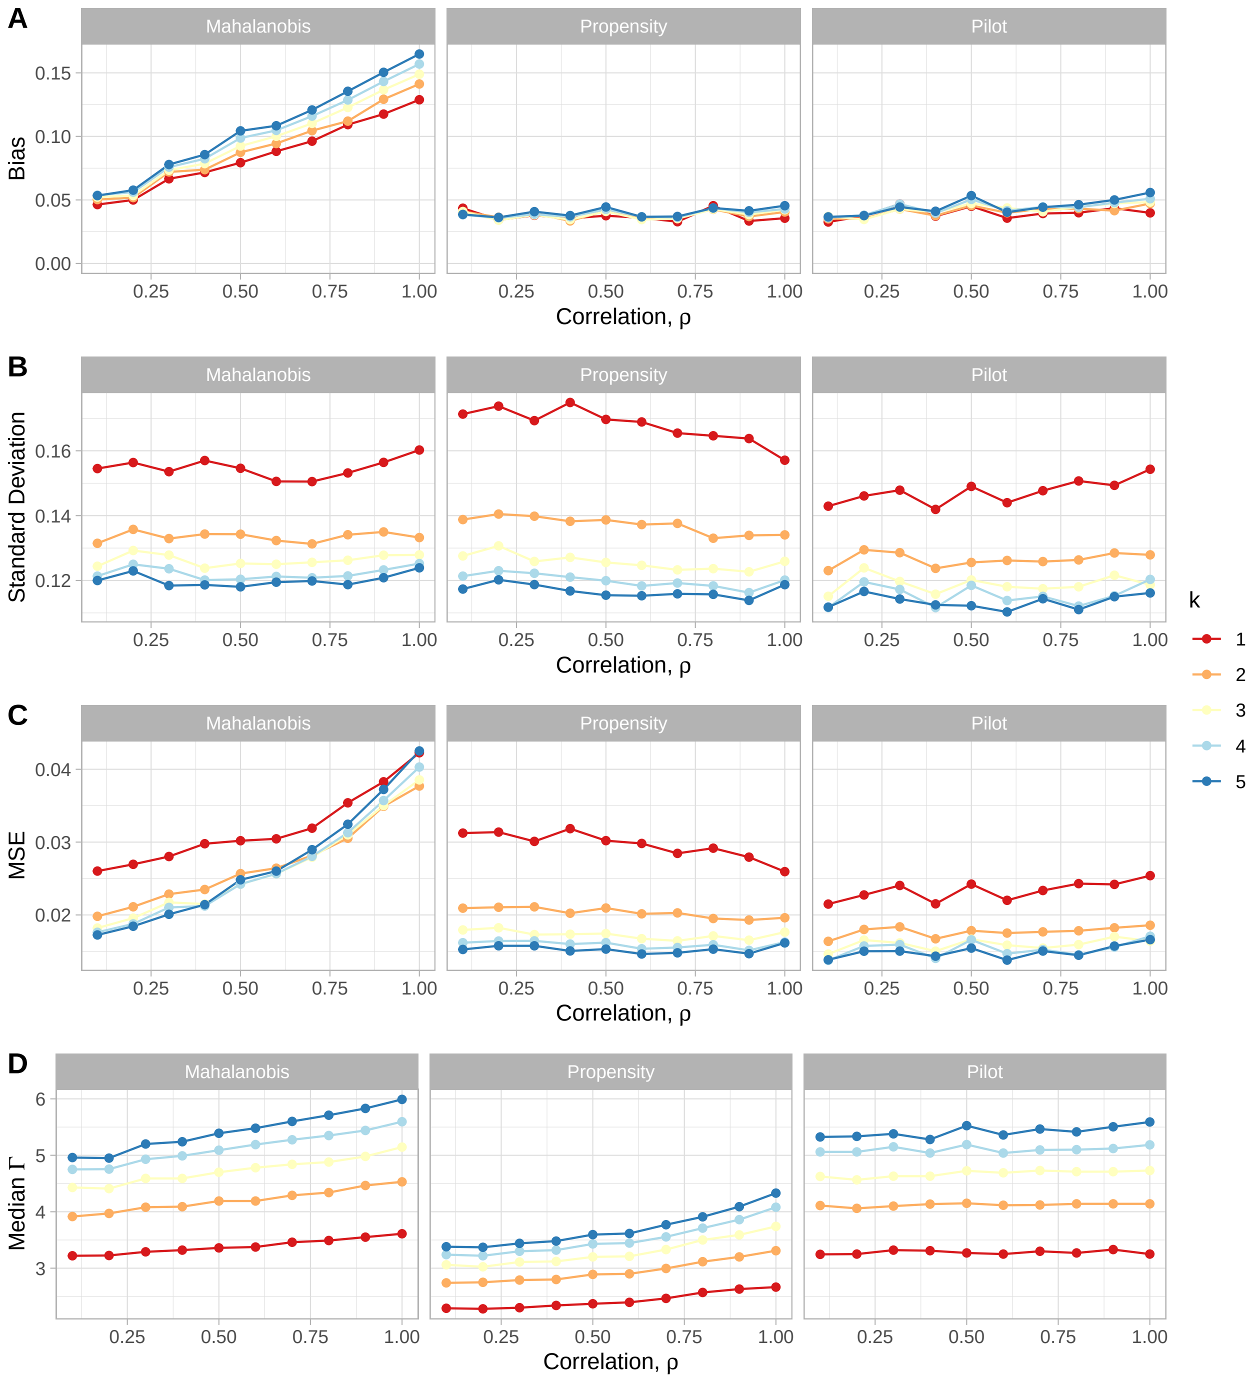


**Supplementary Figure 3:** Bias, standard deviation, MSE, and median Γ of matching estimators when an unobserved confounder is present.

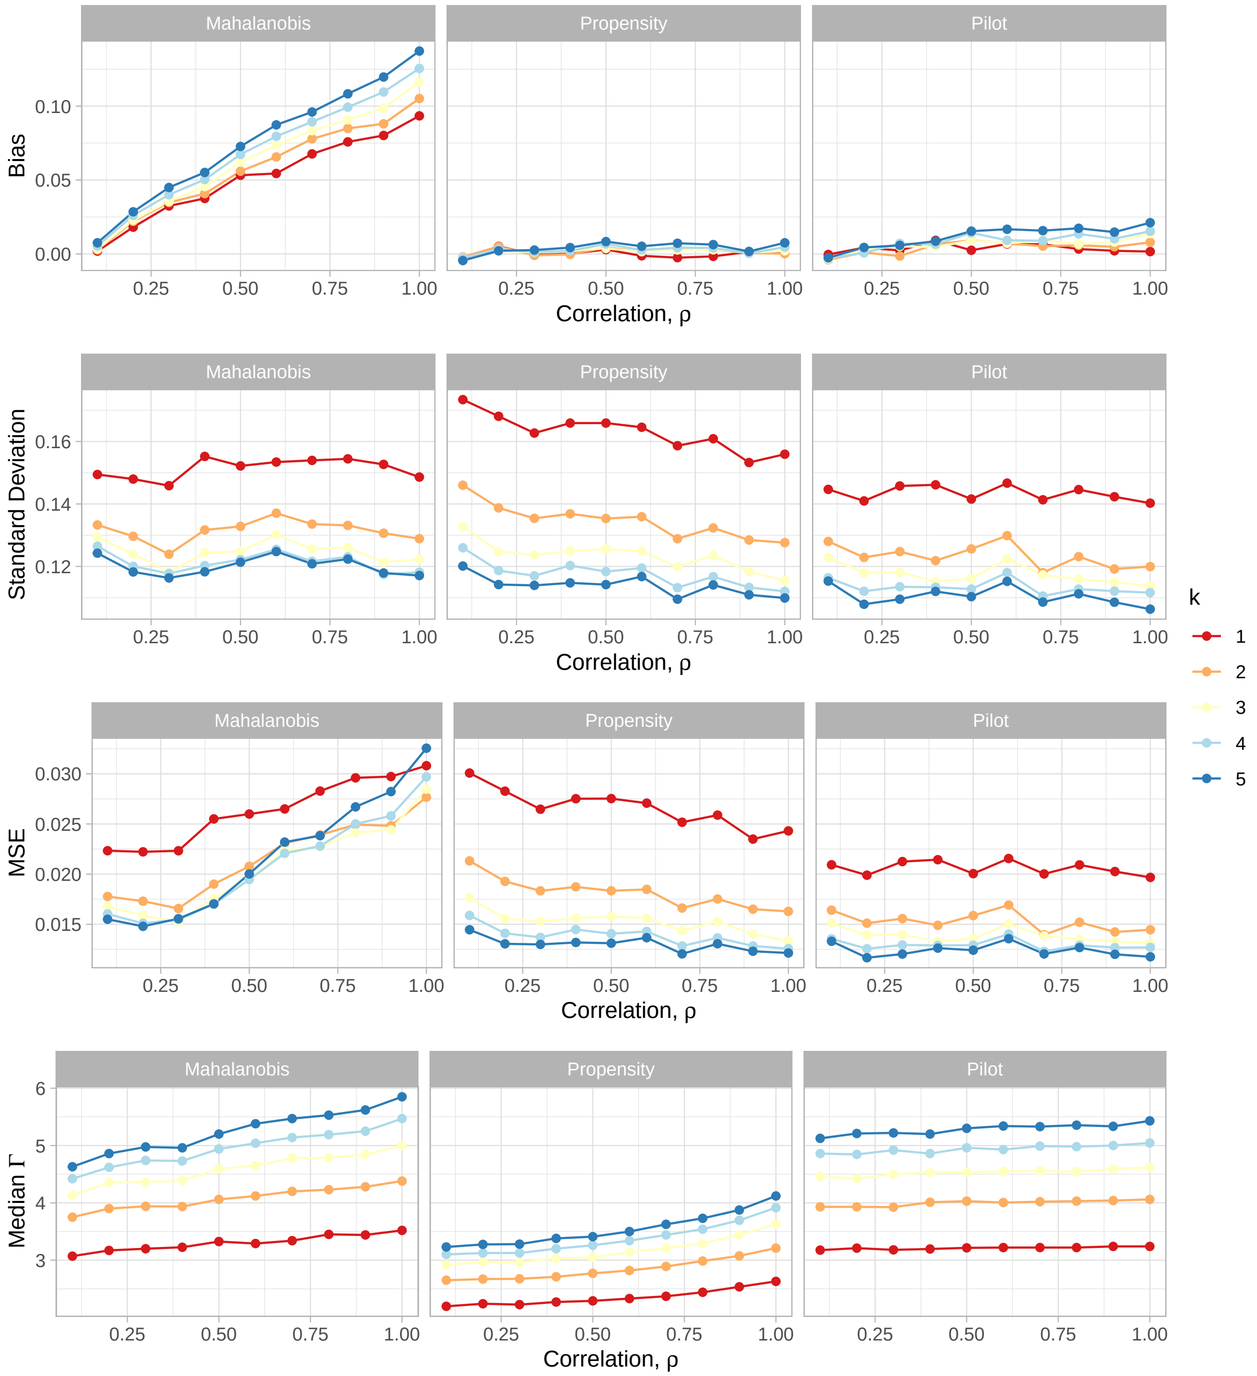


**Supplementary Figure 4:** Mahalanobis, propensity, and prognostic pilot matching performance in terms of Bias (A), Variance (B), and MSE(C) for 1:k optimal matching with a smaller control reserve ($n = 1600$)

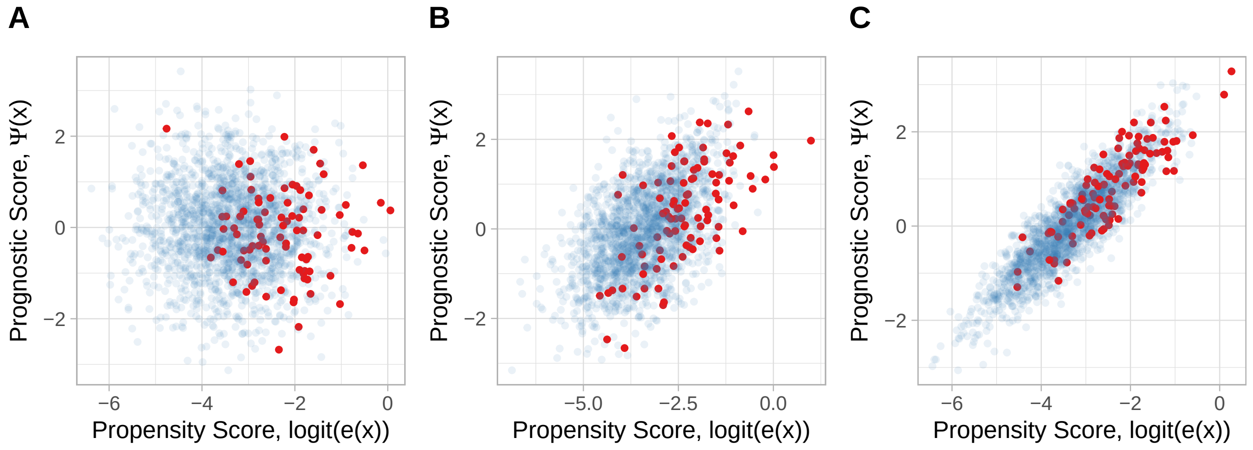


**Supplementary Figure 5:** Example Fisher-Mill plots for a scenario with diminished covariate overlap between treated and control individuals. Blue dots represent control individuals, red dots represent treated individuals, and dotted lines connect matched pairs. The correllation $\rho$ between $\phi$ and $\Psi$ is 0, 0.5, and 0.9, respectively in figures (A), (B) and (C). Simulations were carried out as described in Section 4.2, but with $\phi(X_i) = X_{i1} - 10/3$. This kept the sample size and number of treated individuals constant while increasing the separation of treated and control individuals in terms of the covariate X1.

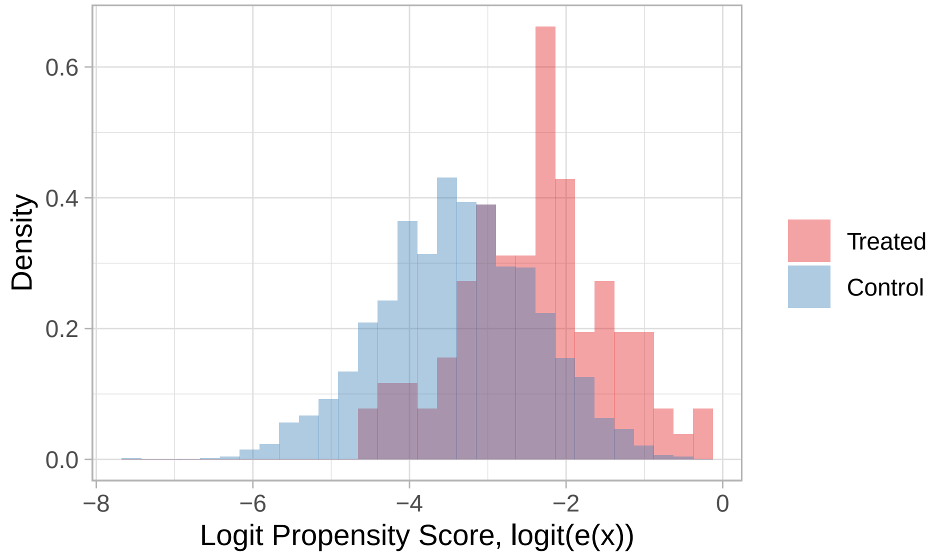


**Supplementary Figure 6:** Example overlayed density plot of logit propensity score in treated and control individuals for a simulation with diminished covariate overlap (in this simulation, $\rho = 0$). Note that there were approximately 19 control observations for every treated observation for each data set, so in practice the counts for the control observations are much larger.

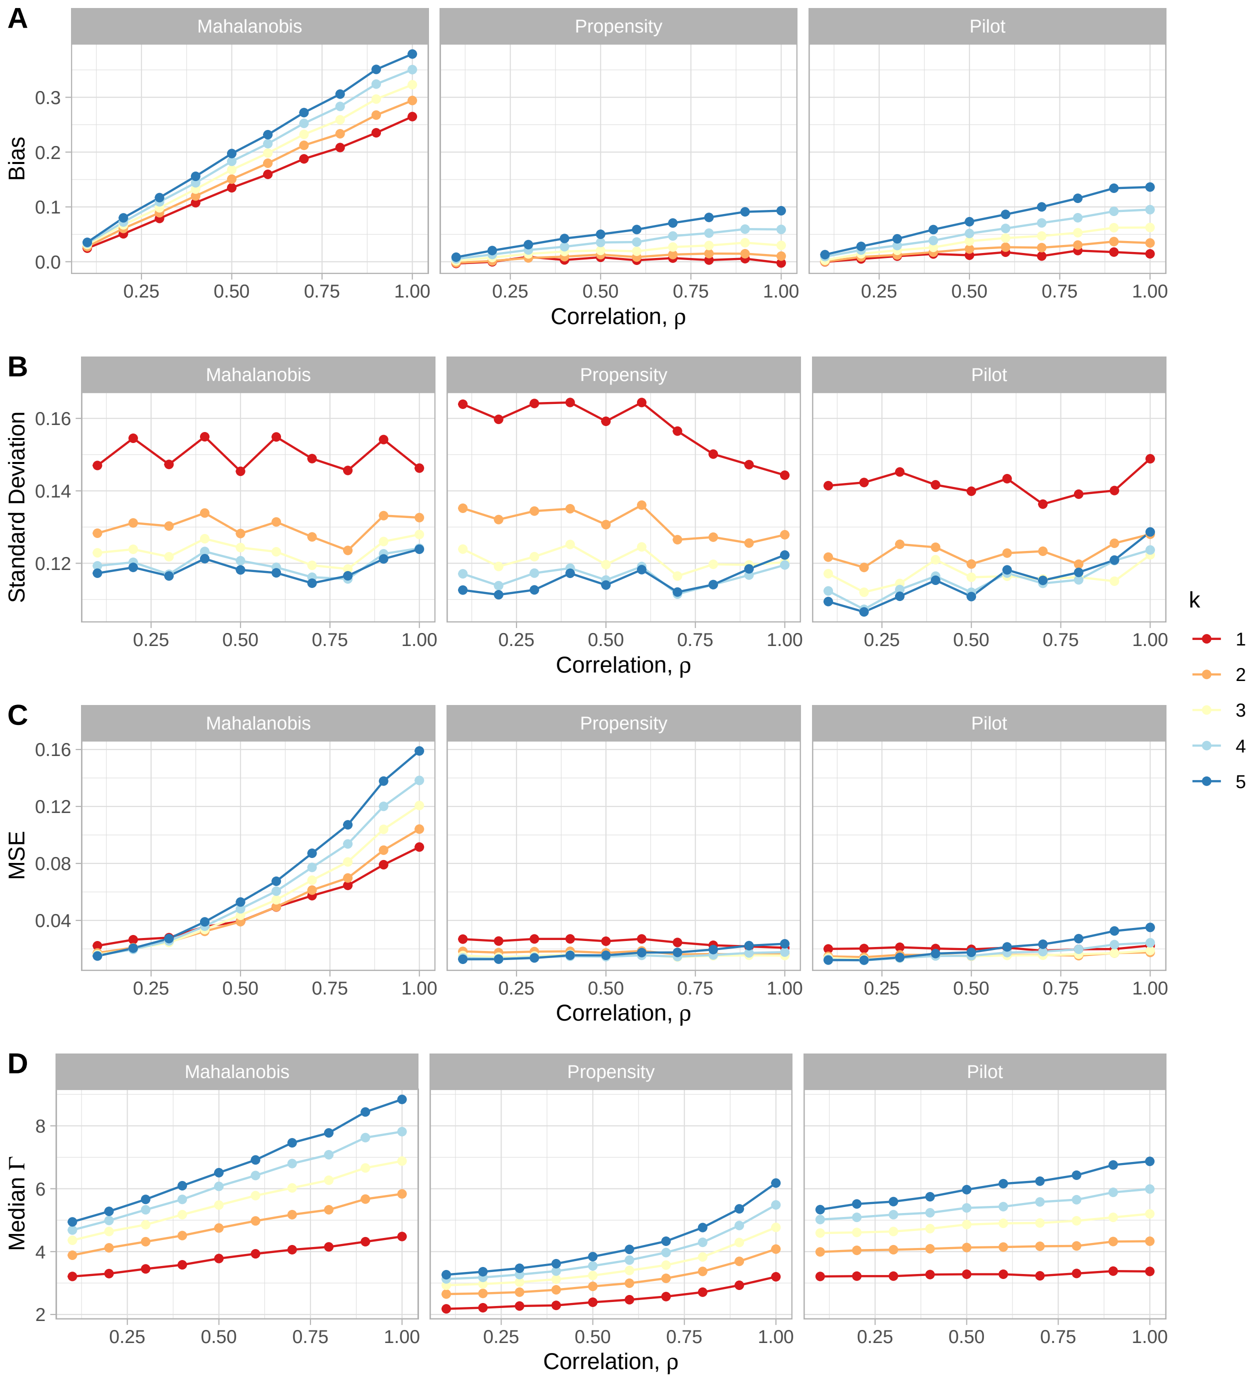


**Supplementary Figure 7:** Bias, standard deviation, MSE, and median Γ from matching estimators for simulations with worse covariate overlap between treated and control observations.

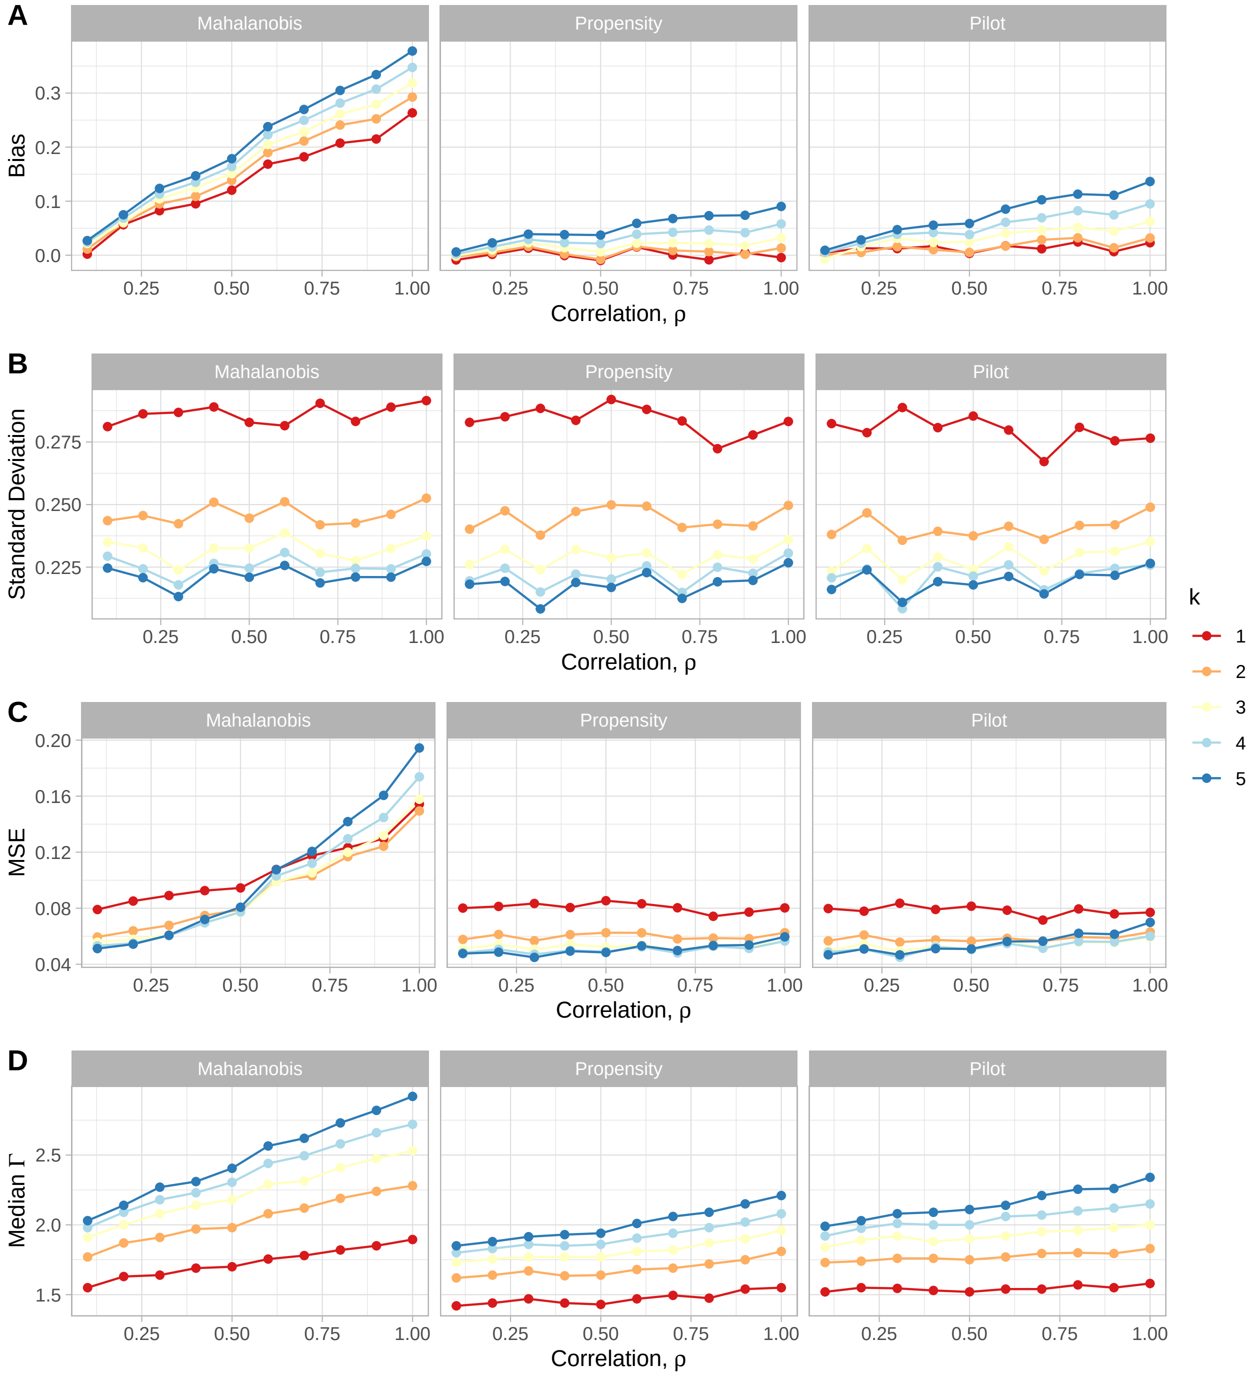


**Supplementary Figure 8:** Bias, standard deviation, MSE and median gamma when the random noise contributing to the outcome is increased. All simulation parameters are the same as described in Section 4.2, except that $\sigma = 2$ This increases the difficulty of fitting the prognostic score, diminishing the relative performance of pilot matching in terms of MSE and sensitivity.

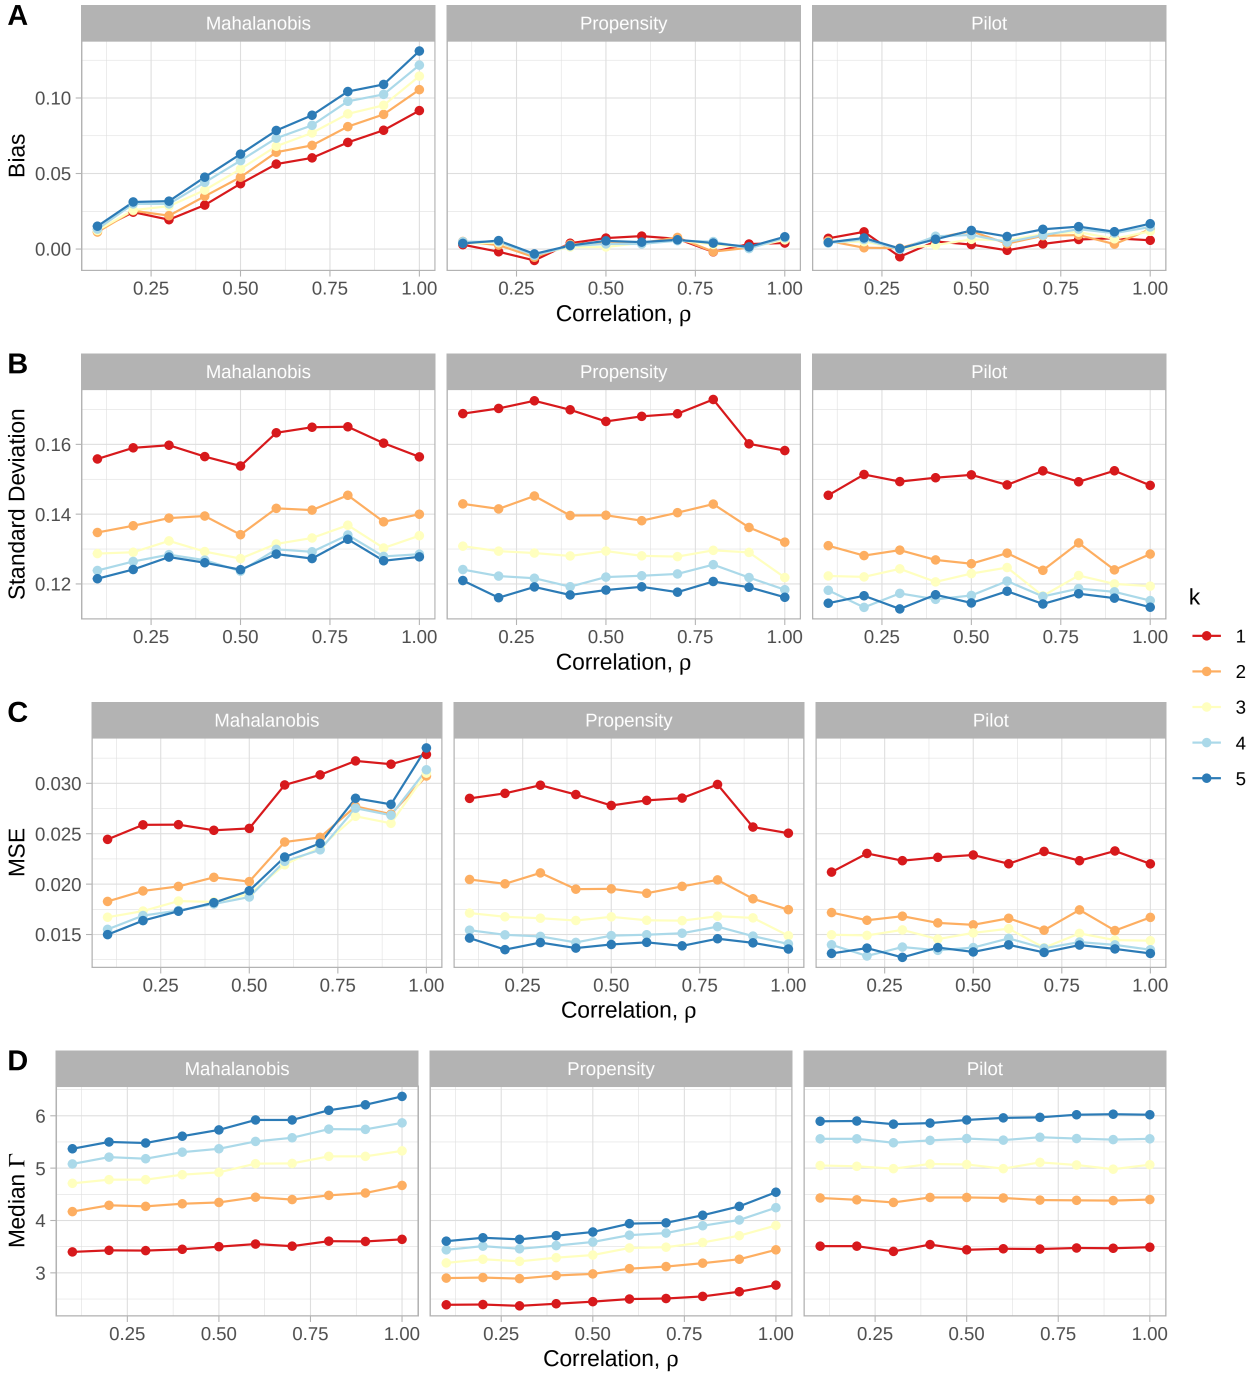


**Supplementary Figure 9:** Bias, standard deviation, MSE, and median Γ from matching estimators for simulations with a heterogeneous treatment effect. Simulations were carried out as described in Section 4.2, but with the individual treatment effect determined by the covariates: $\tau(X_i) = 1 + Xi1/4$.
